# Supplementary material for: Quantum Treatment for Bose-Einstein Condensation in Non-Equilibrium Systems
Source: arXiv:1503.08424 source file (2015-03-29)
Supplement: Supplementary file 1 [file Supplemental_Material.pdf]

# SUPPLEMENTAL MATERIAL

H. Flayac,[1] I. G. Savenko,[2,3] M. Möttönen,[2,4] and T. Ala-Nissila[2,5]

[1]*Institute of Theoretical Physics, Ecole Polytechnique Fédérale de Lausanne (EPFL), CH-1015 Lausanne, Switzerland*
[2]*COMP Centre of Excellence at the Department of Applied Physics, P.O. Box 11000, FI-00076 Aalto, Finland*
[3]*National Research University of Information Technologies, Mechanics and Optics (ITMO University), Saint-Petersburg 197101, Russia*
[4]*QCD Labs, Department of Applied Physics, P.O. Box 13500, FI-00076 Aalto, Finland*
[5]*Department of Physics, P.O. Box 1843, Brown University, Providence, Rhode Island 02912-1843, USA*

In this Supplemental Material we discuss the terms (3) and (4) of the system Hamiltonian from the main text and present an explicit derivation of the quantum jump operators.

### Coupling to the thermal reservoir of acoustic phonons

Taking into account only the energy and momentum conserving terms, the Hamiltonian of the polariton–phonon interaction [Eq. (3) of the main text] reads

$$\begin{aligned}\hat{\mathcal{H}}_{\text{p-ph}} &= \sum_{\mathbf{k}_1,\mathbf{k}_2}\left[\int \frac{L_z dq_z}{2\pi} G_{\mathbf{q}} \hat{a}^\dagger_{\mathbf{k}_1}\hat{a}_{\mathbf{k}_2}\hat{b}_{\mathbf{q}} + \text{h.c.}\right] \qquad (1)\\ &= \frac{L_z}{2\pi}\sum_{\mathbf{k}_1,\mathbf{k}_2;E_{\mathbf{k_1}}>E_{\mathbf{k_2}}}\left(\int_{-\pi/L_z}^{\pi/L_z} dq_z G_{|\mathbf{k}_1-\mathbf{k}_2|,q_z}\hat{a}^\dagger_{\mathbf{k}_1}\hat{a}_{\mathbf{k}_2}\hat{b}_{\mathbf{k}_1-\mathbf{k}_2,q_z}\right)\\ &+ \frac{L_z}{2\pi}\sum_{\mathbf{k}_1,\mathbf{k}_2;E_{\mathbf{k_1}}<E_{\mathbf{k_2}}}\left(\int_{-\pi/L_z}^{\pi/L_z} dq_z G^*_{|\mathbf{k}_1-\mathbf{k}_2|,q_z}\hat{a}^\dagger_{\mathbf{k}_1}\hat{a}_{\mathbf{k}_2}\hat{b}^\dagger_{\mathbf{k}_1-\mathbf{k}_2,q_z}\right).\end{aligned}$$

The scattering strength is given by [1, 2]

$$G_{|\mathbf{k}_1-\mathbf{k}_2|,q_z} = i\sqrt{\frac{\hbar\sqrt{|\mathbf{k}_1-\mathbf{k}_2|^2+q_z^2}}{2\rho V u}}\left[d_e I^e_\parallel(|\mathbf{k}_1-\mathbf{k}_2|)I^e_\perp(q_z) - d_h I^h_\parallel(|\mathbf{k}_1-\mathbf{k}_2|)I^h_\perp(q_z)\right], \qquad (2)$$

where $\rho = 5318$ kg/m$^3$ is the material density, $V$ is the volume of the system which in our case is a quantum well (QW), $u = 3350$ m/s is the speed of sound, $d_e = -7$ eV and $d_h = 2.7$ eV are the deformation potentials of the lattice induced by phonons at the points of location of electrons and holes. The thickness of the QW is $L_z = 10$ nm and the excitonic Bohr radius is $a_\text{B} = 10$ nm. The integrals $I^{e(h)}_\parallel(|\mathbf{k}_1-\mathbf{k}_2|)$ and $I^{e(h)}_\perp(q_z)$ are the overlap integrals of the phonon wave functions with the electron and hole wave functions, respectively, in the in-plane and growth directions, and can be expressed following Ref. [3] as:

$$I^{e(h)}_\parallel(|\mathbf{k}_1-\mathbf{k}_2|) = \left[1+\left(\frac{m_{h(e)}}{m_e+m_h}|\mathbf{k}_1-\mathbf{k}_2|a_\text{B}\right)^2\right]^{-3/2}, \qquad (3)$$

$$I^{e(h)}_\perp(q_z) = \frac{\pi^2}{\frac{q_zL_z}{2}\left(\pi^2-\left(\frac{q_zL_z}{2}\right)^2\right)}\sin\left(\frac{q_zL_z}{2}\right). \qquad (4)$$

Furthermore, we switch to the interaction picture with respect to the free propagation term [the first term in the Hamiltonian (1) in the main text],

$$\hat{a}_{\mathbf{k}}(t) = \hat{a}_{\mathbf{k}}e^{-iE_{\mathbf{k}}t/\hbar}, \quad \hat{a}^\dagger_{\mathbf{k}}(t) = \hat{a}^\dagger_{\mathbf{k}}e^{iE_{\mathbf{k}}t/\hbar}, \qquad (5)$$

and introduce the polariton and reservoir operators:

$$\hat{\mathcal{A}}_{\mathbf{k}_1\mathbf{k}_2}(t) = \hat{a}_{\mathbf{k}_1}\hat{a}^\dagger_{\mathbf{k}_2}e^{-i(E_{\mathbf{k}_1}-E_{\mathbf{k}_2})t/\hbar}, \qquad (6)$$

$$\hat{R}_{\mathbf{k}_1\mathbf{k}_2}(t) = \frac{L_z}{2\pi}\int dq_z G_{|\mathbf{k}_1-\mathbf{k}_2|,q_z}\hat{b}_{|\mathbf{k}_1-\mathbf{k}_2|,q_z}e^{-i\omega_{|\mathbf{k}_1-\mathbf{k}_2|,q_z}t}. \qquad (7)$$

where $\omega_{|\mathbf{k}_1-\mathbf{k}_2|,q_z}$ is the phonon dispersion defined in the main text as $\omega_{\mathbf{q}}$. Then we obtain

$$\hat{\mathcal{H}}_{\text{p-ph}}(t) = \hbar \sum_{\mathbf{k}_1\mathbf{k}_2} \{\hat{\mathcal{A}}_{\mathbf{k}_1\mathbf{k}_2}(t)\hat{R}^{\dagger}_{\mathbf{k}_1\mathbf{k}_2}(t) + \hat{\mathcal{A}}^{\dagger}_{\mathbf{k}_1\mathbf{k}_2}(t)\hat{R}_{\mathbf{k}_1\mathbf{k}_2}(t)\}. \tag{8}$$

## Coupling to the pumping reservoir

Taking into account the energy and momentum conserving terms only, the Hamiltonian corresponding to incoherent pumping [Eq. (4) of the main text] reads

$$\hat{\mathcal{H}}_{\text{pump}} = \hbar \sum_{\mathbf{k}\xi} \left( g_{\mathbf{k}\xi}\hat{a}_{\mathbf{k}}\hat{d}^{\dagger}_{\xi} + g^{*}_{\mathbf{k}\xi}\hat{a}^{\dagger}_{\mathbf{k}}\hat{d}_{\xi} \right) = \hbar \sum_{\mathbf{k}} \left( g_{\mathbf{k}}\hat{a}_{\mathbf{k}}\hat{d}^{\dagger}_{\mathbf{k}} + g^{*}_{\mathbf{k}}\hat{a}^{\dagger}_{\mathbf{k}}\hat{d}_{\mathbf{k}} \right), \tag{9}$$

where in the last equality we assumed that $g_{\mathbf{k}\xi} = g_{\mathbf{k}}$. In terms of the pumping source operators,

$$\hat{D}_{\mathbf{k}}(t) \;=\; g_{\mathbf{k}}\hat{d}_{\mathbf{k}}e^{-iw^{\text{P}}_{\mathbf{k}}t}, \tag{10}$$

in the assumption $w^{\text{P}}_{\mathbf{k}} = E_{\mathbf{k}}$, Eq. (9) turns into

$$\hat{\mathcal{H}}_{\text{pump}}(t) = \hbar \sum_{\mathbf{k}} \{\hat{a}_{\mathbf{k}}(t)\hat{D}^{\dagger}_{\mathbf{k}}(t) + \hat{a}^{\dagger}_{\mathbf{k}}(t)\hat{D}_{\mathbf{k}}(t)\}. \tag{11}$$

## The master equation

The full density operator, $\hat{\chi}$, of the total quantum system (including the subsystem of polaritons and both the phonon and pumping source reservoirs) is subject to the Liouville-von Neumann equation:

$$i\hbar\partial_t\hat{\chi} = [\hat{\mathcal{H}}, \hat{\chi}]. \tag{12}$$

We apply the Born approximation to factorize the density operator as

$$\hat{\chi} = \hat{\rho} \otimes \hat{\rho}^{\text{p-ph}} \otimes \hat{\rho}^{\text{pump}}, \tag{13}$$

where $\hat{\rho}^{\text{p-ph}}$ and $\hat{\rho}^{\text{pump}}$ are the density operators of the phonon and pumping subsystems, respectively. Further, we use the definition of partial trace as

$$\hat{\rho}(t) = \text{Tr}_{\text{pump}}\text{Tr}_{\text{p-ph}}\left\{\hat{\chi}(t)\right\}. \tag{14}$$

Thus the master equation for the system density operator may be written in the interaction picture as

$$\partial_t\hat{\rho}(t) = -\frac{1}{\hbar^2}\int_0^t \text{Tr}_{\text{pump}}\text{Tr}_{\text{p-ph}}[\hat{\mathcal{H}}_{\text{p-ph}}(t) + \hat{\mathcal{H}}_{\text{pump}}(t), [\hat{\mathcal{H}}_{\text{p-ph}}(\tau) + \hat{\mathcal{H}}_{\text{pump}}(\tau), \hat{\chi}(\tau)]]d\tau. \tag{15}$$

We make a reasonable assumption of independence of the pumping reservoir and the phonon reservoir, which yields

$$\begin{aligned}\partial_t\hat{\rho} \;&=\; -\frac{1}{\hbar^2}\int_0^t \text{Tr}_{\text{pump}}[\hat{\mathcal{H}}_{\text{pump}}(t), [\hat{\mathcal{H}}_{\text{pump}}(\tau), \hat{\chi}(\tau)]]d\tau - \frac{1}{\hbar^2}\int_0^t \text{Tr}_{\text{p-ph}}[\hat{\mathcal{H}}_{\text{p-ph}}(t), [\hat{\mathcal{H}}_{\text{p-ph}}(\tau), \hat{\chi}(\tau)]]d\tau \\ &=\; \partial_t\hat{\rho}^{(1)} + \partial_t\hat{\rho}^{(2)}.\end{aligned} \tag{16}$$

After a straightforward derivation in the framework of the secular approximation (neglecting fast-oscillating terms) we find

$$\begin{aligned}\partial_t\hat{\rho}^{(1)} = -\sum_{\mathbf{k}}\int_0^t d\tau \\ &\{\hat{a}_{\mathbf{k}}(t)\hat{a}^{\dagger}_{\mathbf{k}}(\tau)\hat{\rho} - \hat{a}^{\dagger}_{\mathbf{k}}(\tau)\hat{\rho}\hat{a}_{\mathbf{k}}(t)\} \cdot \langle\hat{D}^{\dagger}_{\mathbf{k}}(t)\hat{D}_{\mathbf{k}}(\tau)\rangle_{\text{pump}} \\ &+\{\hat{\rho}\hat{a}_{\mathbf{k}}(\tau)\hat{a}^{\dagger}_{\mathbf{k}}(t) - \hat{a}^{\dagger}_{\mathbf{k}}(t)\hat{\rho}\hat{a}_{\mathbf{k}}(\tau)\} \cdot \langle\hat{D}^{\dagger}_{\mathbf{k}}(\tau)\hat{D}_{\mathbf{k}}(t)\rangle_{\text{pump}} \\ &+\{\hat{a}_{\mathbf{k}}(t)^{\dagger}\hat{a}_{\mathbf{k}}(\tau)\hat{\rho} - \hat{a}_{\mathbf{k}}(\tau)\hat{\rho}\hat{a}^{\dagger}_{\mathbf{k}}(t)\} \cdot \langle\hat{D}_{\mathbf{k}}(t)\hat{D}^{\dagger}_{\mathbf{k}}(\tau)\rangle_{\text{pump}} \\ &+\{\hat{\rho}\hat{a}^{\dagger}_{\mathbf{k}}(\tau)\hat{a}_{\mathbf{k}}(t) - \hat{a}_{\mathbf{k}}(t)\hat{\rho}\hat{a}^{\dagger}_{\mathbf{k}}(\tau)\} \cdot \langle\hat{D}_{\mathbf{k}}(\tau)\hat{D}^{\dagger}_{\mathbf{k}}(t)\rangle_{\text{pump}},\end{aligned} \tag{17}$$

where $\langle \hat{D}^\dagger_{\mathbf{k}}(t)\hat{D}_{\mathbf{k}}(\tau)\rangle_{\text{pump}} = \text{Tr}_{\text{pump}}\{\hat{D}^\dagger(t)\hat{D}(\tau)\hat{\rho}^{\text{pump}}\}$. Assuming that the pumping reservoir is thermalized, we can write

$$\langle \hat{D}^\dagger_{\mathbf{k}}(t)\hat{D}_{\mathbf{k}}(\tau)\rangle_{\text{pump}} = |g_{\mathbf{k}}|^2 e^{iE_{\mathbf{k}}(t-\tau)/\hbar}\overline{n}_{\text{P}}(E_{\mathbf{k}}) = \gamma_{\mathbf{k}}\overline{n}_{\text{P}}(E_{\mathbf{k}})e^{iE_{\mathbf{k}}(t-\tau)/\hbar}, \tag{18}$$

$$\langle \hat{D}_{\mathbf{k}}(t)\hat{D}^\dagger_{\mathbf{k}}(\tau)\rangle_{\text{pump}} = |g_{\mathbf{k}}|^2 e^{-iE_{\mathbf{k}}(t-\tau)/\hbar}\left[\overline{n}_{\text{P}}(E_{\mathbf{k}})+1\right] = \gamma_{\mathbf{k}}\left[\overline{n}_{\text{P}}(E_{\mathbf{k}})+1\right]e^{-iE_{\mathbf{k}}(t-\tau)/\hbar}, \tag{19}$$

where $\overline{n}_{\text{P}}(\omega)$ is the distribution function of the bosons in the pumping source. Repeating the same steps with respect to the phonon reservoir, we come up with the master equation

$$\partial_t\hat{\rho}^{(2)} = -\sum_{\mathbf{k}_1\mathbf{k}_2}\int_0^t d\tau \tag{20}$$

$$\begin{aligned}
&\{\hat{\mathcal{A}}_{\mathbf{k}_1\mathbf{k}_2}(t)\hat{\mathcal{A}}^\dagger_{\mathbf{k}_1\mathbf{k}_2}(\tau)\hat{\rho} - \hat{\mathcal{A}}^\dagger_{\mathbf{k}_1\mathbf{k}_2}(\tau)\hat{\rho}\hat{\mathcal{A}}_{\mathbf{k}_1\mathbf{k}_2}(t)\}\cdot\langle \hat{R}^\dagger_{\mathbf{k}_1\mathbf{k}_2}(t)\hat{R}_{\mathbf{k}_1\mathbf{k}_2}(\tau)\rangle_{\text{p-ph}}\\
&+\{\hat{\rho}\hat{\mathcal{A}}_{\mathbf{k}_1\mathbf{k}_2}(\tau)\hat{\mathcal{A}}^\dagger_{\mathbf{k}_1\mathbf{k}_2}(t) - \hat{\mathcal{A}}^\dagger_{\mathbf{k}_1\mathbf{k}_2}(t)\hat{\rho}\hat{\mathcal{A}}_{\mathbf{k}_1\mathbf{k}_2}(\tau)\}\cdot\langle \hat{R}^\dagger_{\mathbf{k}_1\mathbf{k}_2}(\tau)\hat{R}_{\mathbf{k}_1\mathbf{k}_2}(t)\rangle_{\text{p-ph}}\\
&+\{\hat{\mathcal{A}}_{\mathbf{k}_1\mathbf{k}_2}(t)^\dagger\hat{\mathcal{A}}_{\mathbf{k}_1\mathbf{k}_2}(\tau)\hat{\rho} - \hat{\mathcal{A}}_{\mathbf{k}_1\mathbf{k}_2}(\tau)\hat{\rho}\hat{\mathcal{A}}^\dagger_{\mathbf{k}_1\mathbf{k}_2}(t)\}\cdot\langle \hat{R}_{\mathbf{k}_1\mathbf{k}_2}(t)\hat{R}^\dagger_{\mathbf{k}_1\mathbf{k}_2}(\tau)\rangle_{\text{p-ph}}\\
&+\{\hat{\rho}\hat{\mathcal{A}}^\dagger_{\mathbf{k}_1\mathbf{k}_2}(\tau)\hat{\mathcal{A}}_{\mathbf{k}_1\mathbf{k}_2}(t) - \hat{\mathcal{A}}_{\mathbf{k}_1\mathbf{k}_2}(t)\hat{\rho}\hat{\mathcal{A}}^\dagger_{\mathbf{k}_1\mathbf{k}_2}(\tau)\}\cdot\langle \hat{R}_{\mathbf{k}_1\mathbf{k}_2}(\tau)\hat{R}^\dagger_{\mathbf{k}_1\mathbf{k}_2}(t)\rangle_{\text{p-ph}},
\end{aligned}$$

where assuming that the phonon reservoir is thermalized, we obtain

$$\langle \hat{R}^\dagger_{\mathbf{k}_1\mathbf{k}_2}(t)\hat{R}_{\mathbf{k}_1\mathbf{k}_2}(\tau)\rangle_{\text{p-ph}} = \frac{L_z}{2\pi}\int dq_z|G_{|\mathbf{k}_1-\mathbf{k}_2|,q_z}|^2 e^{i\omega_{|\mathbf{k}_1-\mathbf{k}_2|,q_z}(t-\tau)}\overline{n}_{\text{ph}}(E_{\mathbf{k}_1}-E_{\mathbf{k}_2}), \tag{21}$$

$$\langle \hat{R}_{\mathbf{k}_1\mathbf{k}_2}(t)\hat{R}^\dagger_{\mathbf{k}_1\mathbf{k}_2}(\tau)\rangle_{\text{p-ph}} = \frac{L_z}{2\pi}\int dq_z|G_{|\mathbf{k}_1-\mathbf{k}_2|,q_z}|^2 e^{-i\omega_{|\mathbf{k}_1-\mathbf{k}_2|,q_z}(t-\tau)}\left[\overline{n}_{\text{ph}}(E_{\mathbf{k}_1}-E_{\mathbf{k}_2})+1\right]. \tag{22}$$

In the framework of the approximation $G_{|\mathbf{k}_1-\mathbf{k}_2|,q_z} = G_0$, we can further write

$$\langle \hat{R}^\dagger_{\mathbf{k}_1\mathbf{k}_2}(t)\hat{R}_{\mathbf{k}_1\mathbf{k}_2}(\tau)\rangle_{\text{p-ph}} = \gamma^{\text{ph}}_{\mathbf{k}_1\mathbf{k}_2}\overline{n}_{\text{P}}(E_{\mathbf{k}_1}-E_{\mathbf{k}_2})\frac{L_z}{2\pi}\int dq_z e^{i\omega_{|\mathbf{k}_1-\mathbf{k}_2|,q_z}(t-\tau)}, \tag{23}$$

$$\langle \hat{R}_{\mathbf{k}_1\mathbf{k}_2}(t)\hat{R}^\dagger_{\mathbf{k}_1\mathbf{k}_2}(\tau)\rangle_{\text{p-ph}} = \gamma^{\text{ph}}_{\mathbf{k}_1\mathbf{k}_2}\left[\overline{n}_{\text{P}}(E_{\mathbf{k}_1}-E_{\mathbf{k}_2})+1\right]\frac{L_z}{2\pi}\int dq_z e^{-i\omega_{|\mathbf{k}_1-\mathbf{k}_2|,q_z}(t-\tau)}. \tag{24}$$

Executing the temporal integrals in Eqs. (17) and (20), we obtain a Lindblad master equation with the quantum jump operators presented in the main text in Eqs. (5)–(8).


[1] F Tassone, C Piermarocchi, V Savona, A Quattropani, & P Schwendimann, Phys. Rev. B, **56**, 7554 (1997).
[2] V E Hartwell & D W Snoke, Phys. Rev. B, **82**, 075307 (2010).
[3] C. Piermarocchi, F. Tassone, V. Savona, A. Quattropani and P. Schwendimann, Phys. Rev. B **53** (23) 15834 (1996).
[4] F. Tassone and Y. Yamamoto, Phys. Rev. B **59** (16), 10830 (1999).
[5] E. Yu. Perlin, T. A. Vartanian, A. V. Fedorov (Solid State Physics [Rus: Fizika Tverdogo Tela], Saint-Petersburg 2008).
[6] I. Carusotto and C. Ciuti, Phys. Rev. Lett., **93**, 166401 (2004).
[7] K. Mölmer et al., J. Opt. Soc. Am. B **10** (3) (1993); J. Dalibard et al., Phys. Rev. Lett. **68** (5) p. 580 (1992).
